# Supplementary material for: PipeNet: Question Answering with Semantic Pruning over Knowledge Graphs
Source: arXiv:2401.17536 source file (2024-05-17)
Supplement: Supplementary file 1 [file 7-appendix.tex]

\clearpage

\appendix

\section{Appendix}

\subsection{Accuracy score with pruning rate}
\label{appen:1}

\begin{table}[t]
\small\centering
\begin{tabular}{p{0.6cm}p{0.22cm}p{0.22cm}p{0.22cm}p{0.22cm}p{0.22cm}p{0.22cm}p{0.22cm}p{0.22cm}p{0.22cm}p{0.22cm}}
\toprule
$p$(\%) & 2-hop & 10 & 20 & 30 & 40 & 50 & 60 & 70 & 80 & 90 \\
\midrule
%$k$ & 1.0 & 1.07 & 1.16 & 1.26 & 1.41 & 1.62 & 1.93 & 2.39 & 3.24 & 4.78 \\
$k$ & 1.0 & 1.1 & 1.2 & 1.3 & 1.4 & 1.6 & 2.0 & 2.4 & 3.2 & 4.8 \\
\midrule
$M$(G) & 11.5 & & & & & & & & & 4.8 \\ 
$\uparrow$(\%) & - & & & & & & & & & 240 \\
\midrule
$t$(s) & 0.93 & & & & & & & & & 0.52 \\
$\uparrow$(\%) & - & & & & & & & & & 178 \\
\bottomrule
\end{tabular}
\caption{Results on CommonsenseQA in-house split with PipeNet. The pre-trained model is RoBERTa-Large. Time efficiency improvement with pruning rate $p$. Training batch size is 64 on CSQA. }
\label{App:1}
%\vskip-1.0em
\end{table}

\begin{figure}[t]
\centering
\includegraphics[scale=0.5, trim={1cm 0 0cm 1cm}]{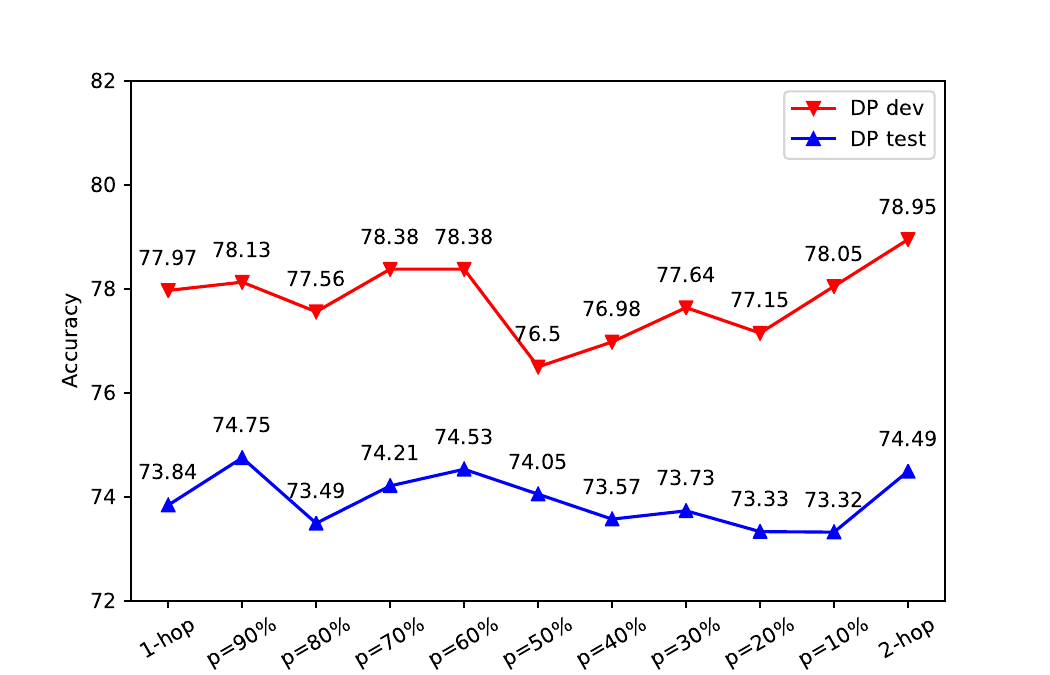}
\caption{Results of DP-pruning method with different pruning rates on external nodes from one-hop to two-hop. Accuracies on CommonsenseQA dev and test split are reported.}
\vskip-1.0em
\label{fig:prune-rate}
\end{figure}

Between one-hop and two-hop, the performances on dev and test split generally are better with $p \geq 60\%$ than those with $ 20\% \leq p <60\% $. It shows that a larger pruning rate can highlight the effectiveness of the DP-pruning strategy because more diverse subgraphs are obtained after the pruning. In the two-hop subgraph, there are about 110 nodes and 2133 edges for each QA context, almost five times to the number of nodes and edges in the subgraph with $p=90\%$. Though more nodes and edges are acquired, the noisy nodes greatly interfere with the subgraph representation learning, leading to a very slight increment on the final performance. Future research on how to utilize informative nodes for subgraph representation learning is worth exploring.

\subsection{Random pruning}

When retrieve hop grows from one to two, more knowledge help. This finding is consistent with the results in GconAttn \cite{2019Improving}, RN \cite{2017A}, and MHGRN \cite{feng2020scalable}. However, the performance gain comes with huge computation and memory costs because many noisy nodes are induced during the expansion process.

With a DP-pruning strategy and pruning rate of 90\%, only comparable amount nodes to one-hop nodes are added while it achieves obvious performance gain over the test set of CSQA and OBQA compared to one-hop. On CSQA, the performance on the test split even outperforms PipeNet with a two-hop subgraph.

\begin{table}[t]
\small\centering
\begin{tabular}{p{0.5cm}p{0.8cm}p{0.6cm}p{1.8cm}p{1.8cm}}
\toprule
$h$-hop & Prune method & Prune rate & RoBERTa-large & AristoRoBERTa \\
\midrule
One & - & 0 & 68.07 ($\pm 1.55$)  &  87.00 ($\pm 0.33$)  \\
Two & - & 0 & 69.33 ($\pm 1.60$)  &  87.33 ($\pm 0.19$)  \\
\midrule
Two & Random & \textbf{90\%} & 68.50 ($\pm 2.50$)  & 87.46 ($\pm 0.55$) \\
Two & DP & \textbf{90\%} & \textbf{69.60} ($\pm 0.47$) & \textbf{87.80}($\pm 0.46)$  \\
\bottomrule
\end{tabular}
\caption{Test accuracy comparison on OpenBookQA with PipeNet. The pre-trained model is RoBERTa-Large and AristoRoBERTa.}
\label{App:2}
\vskip-1.0em
\end{table}
